# Supplementary material for: Collapse modes in SC and BCC arrangements of elastic beads
Source: arXiv:2004.11888 ancillary file (2020-04-13)
Supplement: Supplementary file 1 [file supplementary_material.pdf]

# Collapse modes in SC and BCC arrangements of elastic beads - Supplementary material

Igor A. Ostanin, Artem R. Oganov, Vanessa Magnanimo

April 13, 2020

Below we provide the images of the packings of spherical particles under pressure, observed in our simulations. Particle sizes are shown to scale. We use 2D projections in order to display particle arrangements at surfaces of specimens. Whenever convenient, we utilize the color legend reflecting absolute translational velocities of particles at the final step of the relaxation, which helps identifying separate grains and their relative motion.

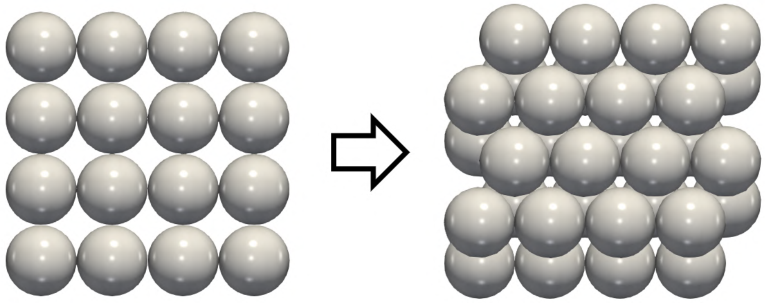

Figure 1: Transformation of $4 \times 4 \times 4$ SC supercell to a defect-free HCP arrangement.

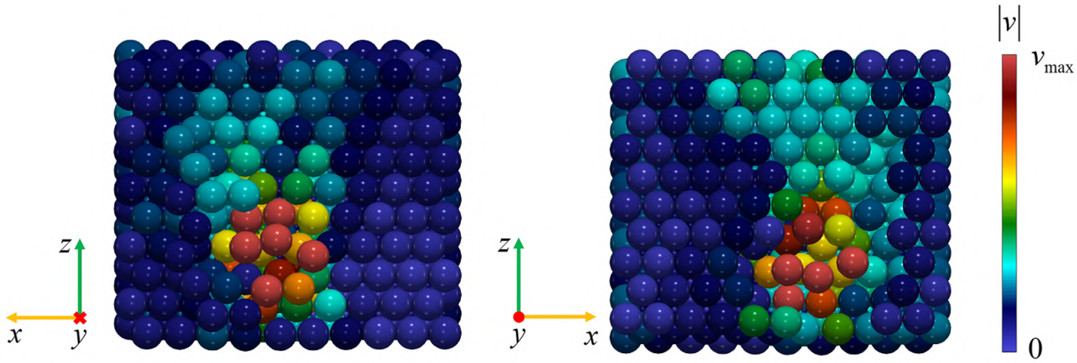


Figure 2: A collapsed $10 \times 10 \times 10$ SC supercell featuring amorphous and HCP regions.

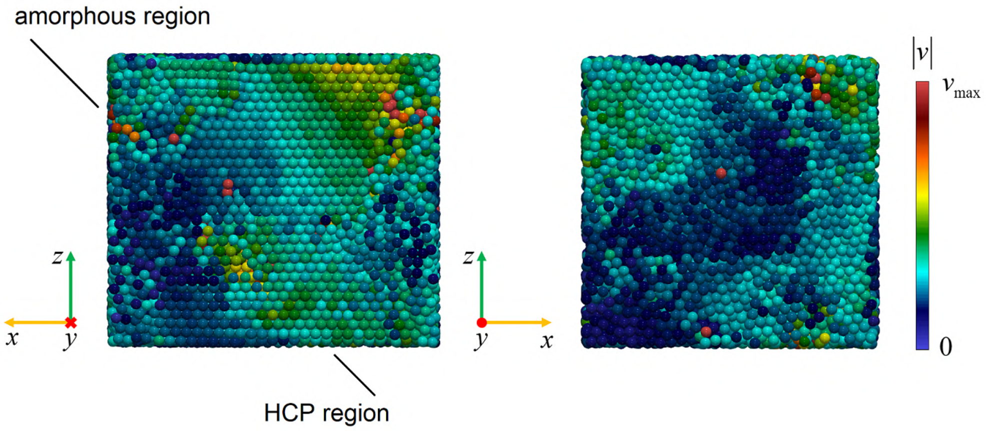


Figure 3: A collapsed 30 × 30 × 30 SC supercell. Amorphous regions, as well as crystalline HCP grains are clearly identifiable.

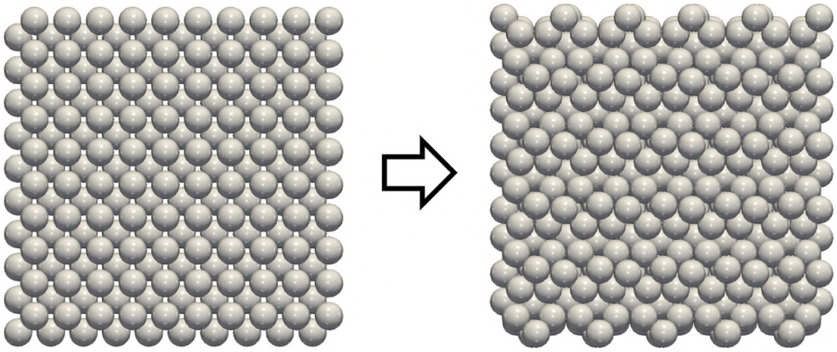

Figure 4: Transformation of 10 × 10 × 10 BCC supercell to a defect-free cI16 arrangement.

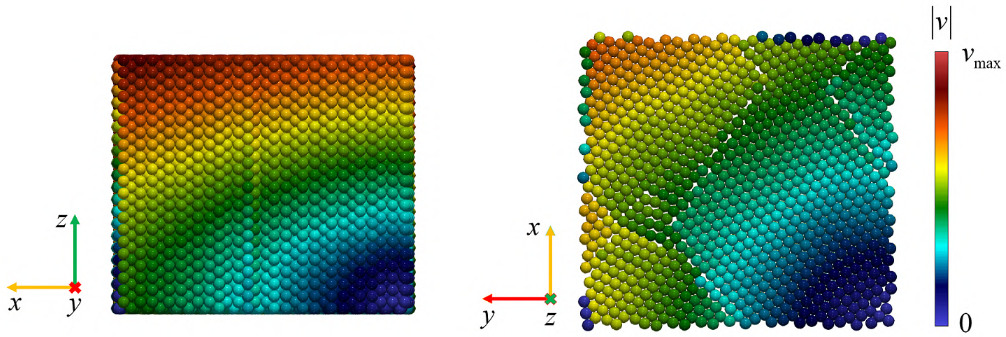


Figure 5: A collapsed 21 × 21 × 21 BCC supercell, featuring defective prismatic SH grains.

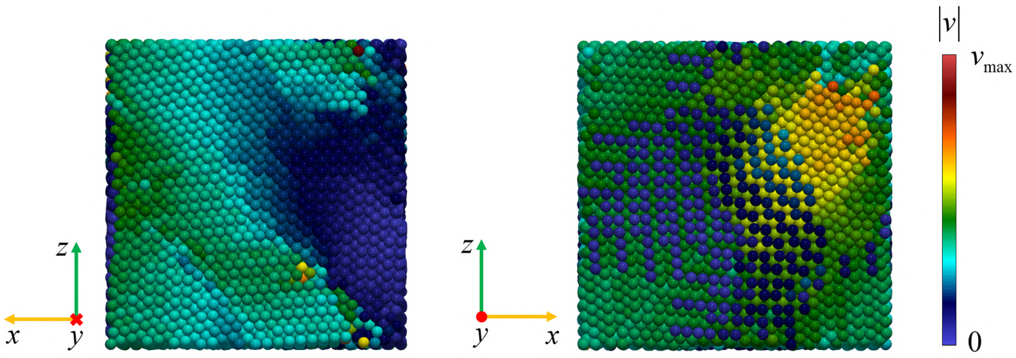


Figure 6: A collapsed 23 × 23 × 23 BCC supercell, displaying multiple cI16 grains.

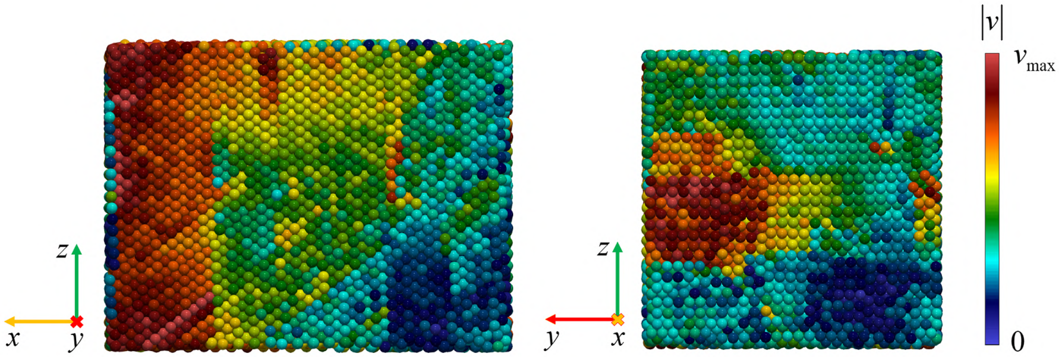


Figure 7: A collapsed 26 × 26 × 26 BCC supercell, showing defective FCC packing.

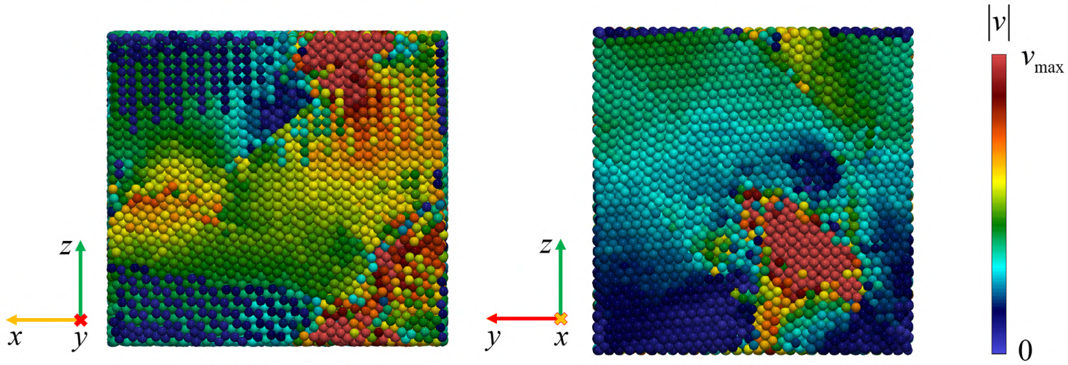


Figure 8: A collapsed 29×29×29 BCC supercell. One can see BCC grains stabilized by surrounding cI16 grains.

## Supplementary videos

- Video 1: transformation of 4 x 4 x 4 SC supercell into defect-free HCP structure.

  `https://youtu.be/uHd9dgGfg80`

- Video 2: Transformation of 10 x 10 x 10 BCC supercell into cI16 arrangement.

  `https://youtu.be/xYbAQAGN1Cs`

- Video 3: Transformation of 12 x 12 x 12 BCC arrangement into FCC arrangement via Bain path.

  `https://youtu.be/jdTk2ZYtjHM`
